# Supplementary material for: Proton dynamics in high-pressure ice-VII from density functional theory
Source: arXiv:2102.11810 ancillary file (2021-02-23)
Supplement: Supplementary file 1 [file ice_vii_sup.pdf]

# Supplementary Material:
# Proton dynamics in high-pressure ice-VII from density functional theory

Florian Trybel,[1,*] Michael Cosacchi,[2] Thomas Meier,[1] Vollrath Martin Axt,[2] and Gerd Steinle-Neumann[1]

[1]*Bayerisches Geoinstitut, Universität Bayreuth, D-95440 Bayreuth, Germany*
[2]*Theoretische Physik III, Universität Bayreuth, D-95440 Bayreuth, Germany*

(Dated: November 1, 2020)

PACS numbers: 71.15.Mb, 63.20.dk, 61.50.Ks,62.50.-p

### Potential Sampling

We trace the potential by displacing collectively all, six and a single proton along the diagonal oxygen-oxygen direction (dOOd). Resulting potentials (shifted to a common energetic zero) for different lattice constants (discussed in detail in the main text) can be found in Figures S1-S5.

### Numerical Approach to Solving Schrödinger's Equation for Proton Tunnelling

A python program is used to calculate the tunnelling frequencies solving the time-dependent Schrödinger equation in one dimension (1D) for a particle in an arbitrary potential. It is inspired by the pySchrodinger `https://github.com/jakevdp/pySchrodinger` code of Jake Vanderplas [1], but uses a matrix exponential formalism instead of a Fourier solver for the time propagation of the wave-function:

$$\Psi(x_\mathrm{i}, t_{\mathrm{i}+1}) = \exp\left(-\frac{\mathrm{i}}{\hbar}\mathcal{H}(x_\mathrm{i})\Delta t\right)\Psi(x_\mathrm{i}, t_\mathrm{i}), \qquad (1)$$

with

$$\mathcal{H} = -\frac{\hbar^2}{2m_\mathrm{p}}\mathcal{D}(x_\mathrm{i}) + \Phi(x_\mathrm{i}), \qquad (2)$$

where $\mathcal{D}$ is the matrix representation of the 3rd order central difference scheme with a stencil reduction at the boundaries, and $\Phi$ the diagonal matrix constructed from the 1D potential and its continuously differentiable continuation. In each $t$-step, the probability of finding the proton in the left half of the double-well potential $p(x < 0) = \int_{-\infty}^{0} |\Psi(x)|^2 dx$ is calculated, and energy as well as norm conservation is checked.

### The Potential

The volume-dependent potential seen by the proton ($\phi_\mathrm{x}(V_\mathrm{i}, x_\mathrm{i})$) is calculated stepwise for different cells, where the respective number of protons is moved to position $x_\mathrm{i}$ along dOOd. The calculated energies per proton are interpolated via a cubic spline, leading to $\phi^s_\mathrm{x}(V_\mathrm{i}, x)$. At small O-H distances (high energies), the DFT calculations do not reliably converge, therefore $\phi^s_\mathrm{x}(V_\mathrm{i}, x)$ is extended using a 1D approximation to the Pauli-repulsion potential $\phi_\mathrm{P}$ at small inter-ionic distances, such that the potential is twice continuously differentiable. We approximate $\phi_\mathrm{P}$ as

$$\phi_\mathrm{P} = \left(\frac{\alpha}{x - x_0}\right)^{12}. \qquad (3)$$

In order to construct a continuously differentiable continuation of the spline, it is necessary to satisfy the conditions

$$\phi^s_\mathrm{x}(\pm x_\mathrm{m}) = \phi_\mathrm{P}(\pm x_\mathrm{m}), \qquad (4a)$$

$$\left.\frac{\partial \phi^s_\mathrm{x}(x)}{\partial x}\right|_{\pm \mathrm{x_m}} = \left.\frac{\partial \phi_\mathrm{P}(x)}{\partial x}\right|_{\pm \mathrm{x_m}}, \qquad (4b)$$

where $\pm x_\mathrm{m}$ is the last point at which $\phi^s_\mathrm{x}$ is calculated explicitly. This leads to parameters $\alpha$ and $x_0$ in equation (3):

$$\alpha = \mp 12\left(\left.\frac{\partial \phi^s_\mathrm{x}(x)}{\partial x}\right|_{\pm \mathrm{x_m}}\right)^{-1} \phi^s_\mathrm{x}(\pm x_\mathrm{m})^{13/12}, \qquad (5a)$$

$$x_0 = \pm x_\mathrm{m} \pm 12\left(\left.\frac{\partial \phi^s_\mathrm{x}(x)}{\partial x}\right|_{\pm \mathrm{x_m}}\right)^{-1} \phi^s_\mathrm{x}(\pm x_\mathrm{m}). \qquad (5b)$$

### Initial State

In order to improve the localization of the initial state described in equation (1) of the main text, a mollifier of the form

$$\mathcal{F}(z) = \begin{cases} \frac{1}{c_\mathrm{n}}\exp((z^2-1)^{-1}), & \text{if } |z| < 1, \\ 0, & \text{if } |z| \geq 1, \end{cases} \qquad (6)$$

with $z = \frac{x - x_0}{3a}$ and $c_\mathrm{n}$ ensuring normalization of $\mathcal{F}(z)$, is used, and the proton is then represented by

$$\Psi(V, T, x) = \mathcal{I}^{-1} \cdot \mathcal{F}(\frac{x - x_0}{3a}) \cdot \mathcal{G}(V, T, x), \qquad (7)$$

$$\mathcal{I} = \int_X \left|\mathcal{F}(\frac{x - x_0}{3a}) \cdot \mathcal{G}(V, T, x)\right|^2 dx. \qquad (8)$$

* f.trybel@uni-bayreuth.de

[1] WRF Data Science Studio, University of Washington.
[2] L. Lin, J. A. Morrone, and R. Car, Journal of Statistical Physics **145**, 365 (2011).
[3] C. Drechsel-Grau and D. Marx, Physical Chemistry Chemical Physics **19**, 2623 (2017).

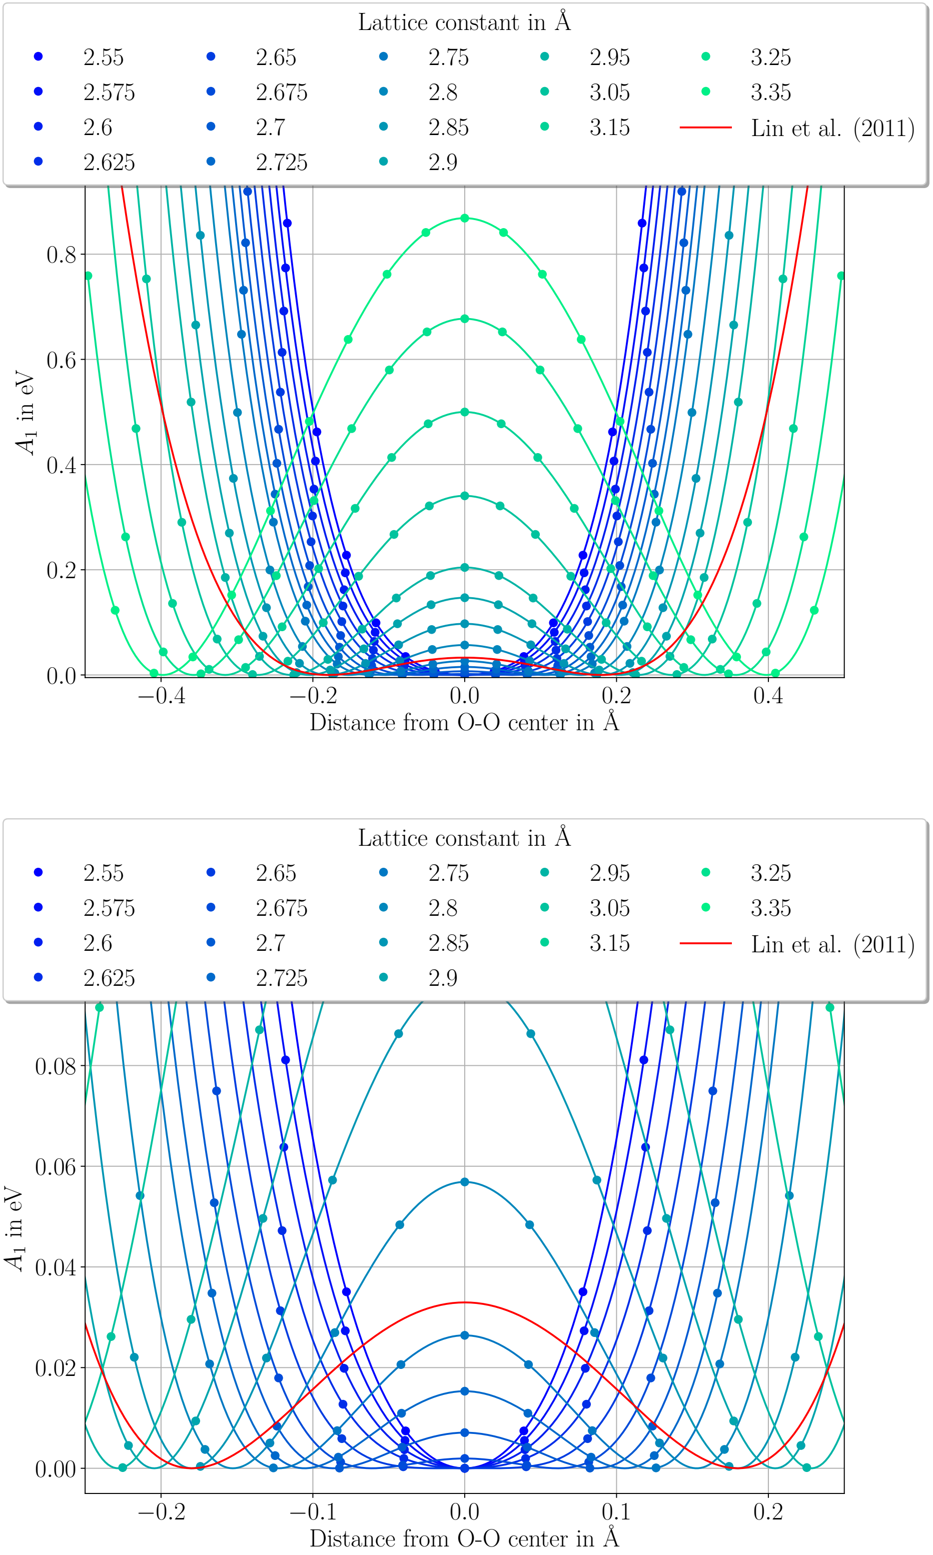


FIG. S1. Potentials obtained by collectively sampling all protons along dOOd. **(top)** The barrier in the double-well potential decreases with decreasing lattice constant (increasing compression) until the double-well character is lost at a lattice constant $l \lesssim 2.675$ Å. **(bottom)** Rescaling the y-axis, we can see that the potentials continuously merge to a single-well with compression. During this process minima in the potential move closer to the center. The potential of Lin *et al.* [2] at 2.84 Å (red) is shown for comparison

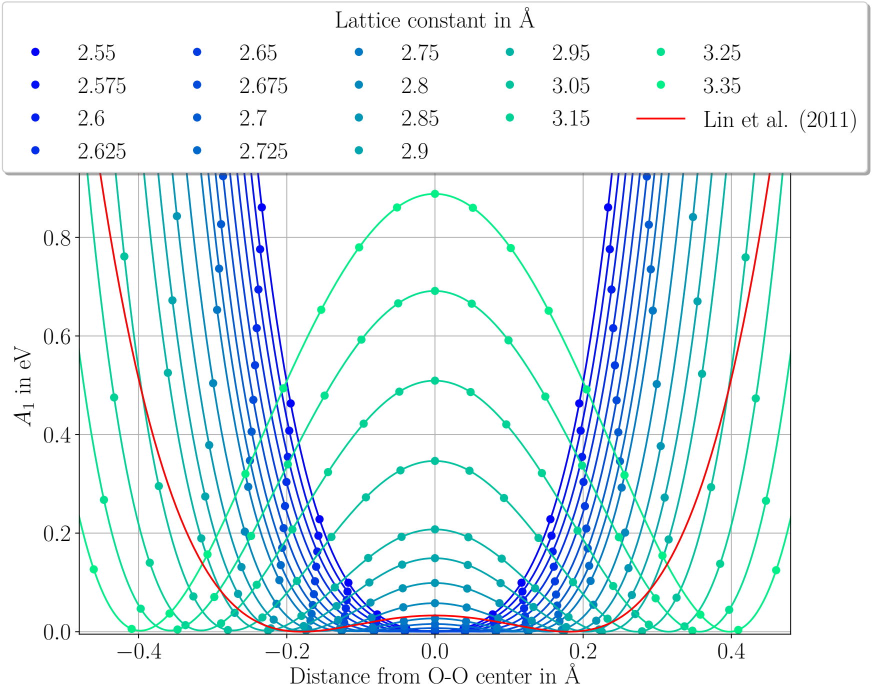


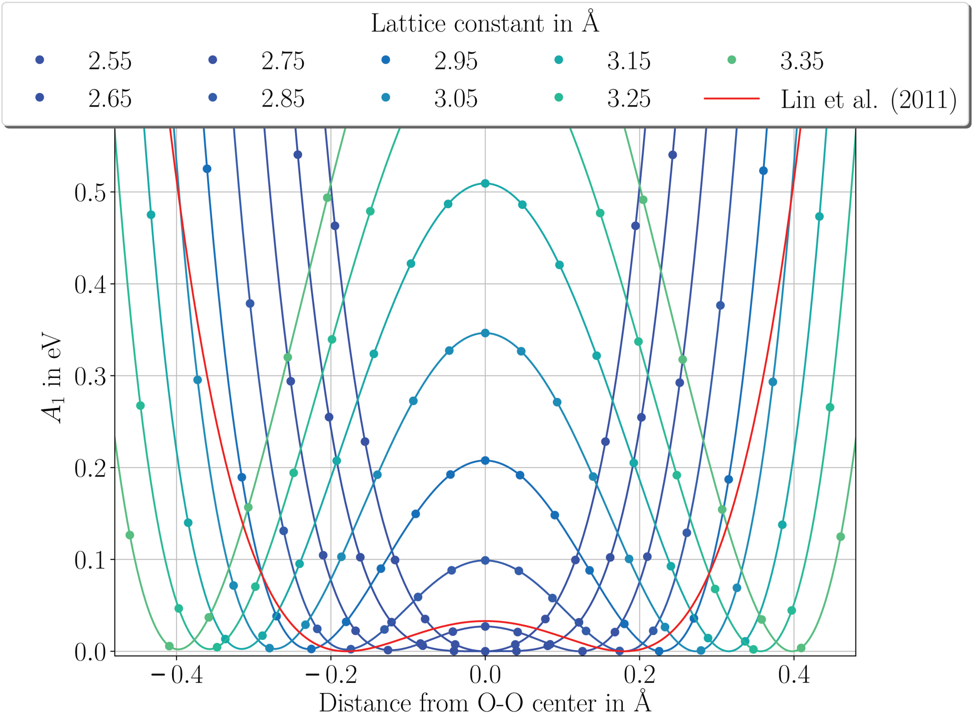


FIG. S2. Potentials of proton positions along dOOd, when six protons are shifted simultaneously in a hexagonal configuration as suggested by Lin *et al.* [2] and Drechsel-Grau and Marx [3]. **(top)** All sampled lattice constants and **(bottom)** and a reduced set of results (zooming in on a smaller energy scale). With compression, the distance between the minima and the height of the barrier decreases until for lattice constant of $l \lesssim 2.675$ Å the double-well character is lost. The form of the potentials is nearly equal to Figure S1, with a slight asymmetry due to the non-central position of the hexagon in the simulation cell (reflecting the effects of the periodic boundary conditions). The potential of Lin *et al.* [2] at 2.84 Å is shown in red.

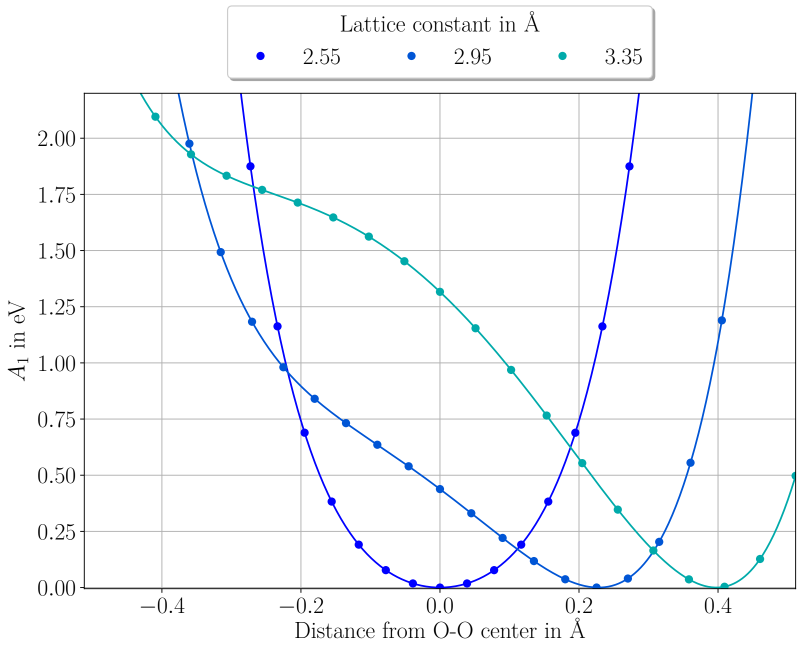


FIG. S3. Potentials obtained by sampling a single proton along dOOd in an ice-rule conforming configuration. The potential is strongly asymmetric with the minima closely matching one of the minima for the cases of the collectively all and hexagonal configurations. With compression, the asymmetry decreases and the potential approximates the cases for the collectively all/hexagonal configurations, with a slightly more pronounced localization.

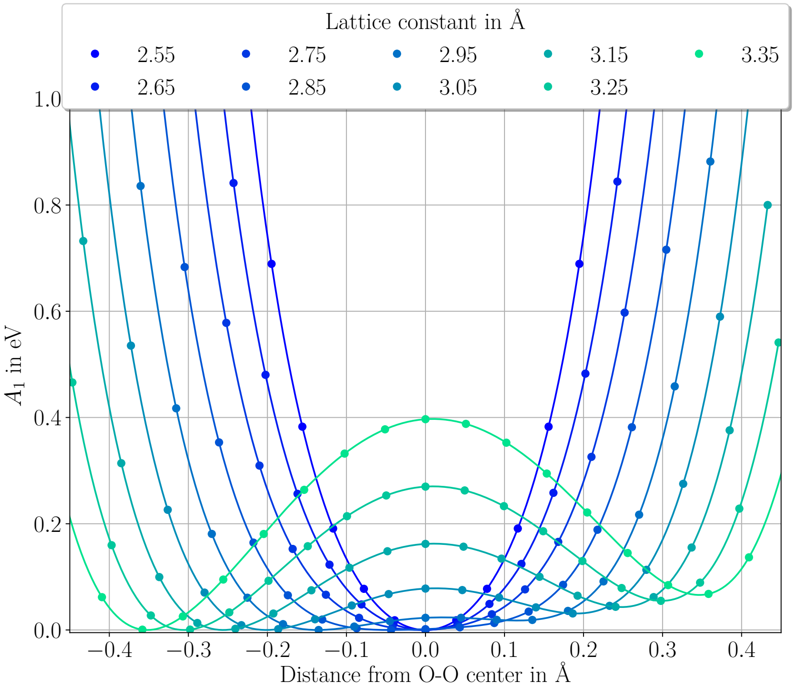


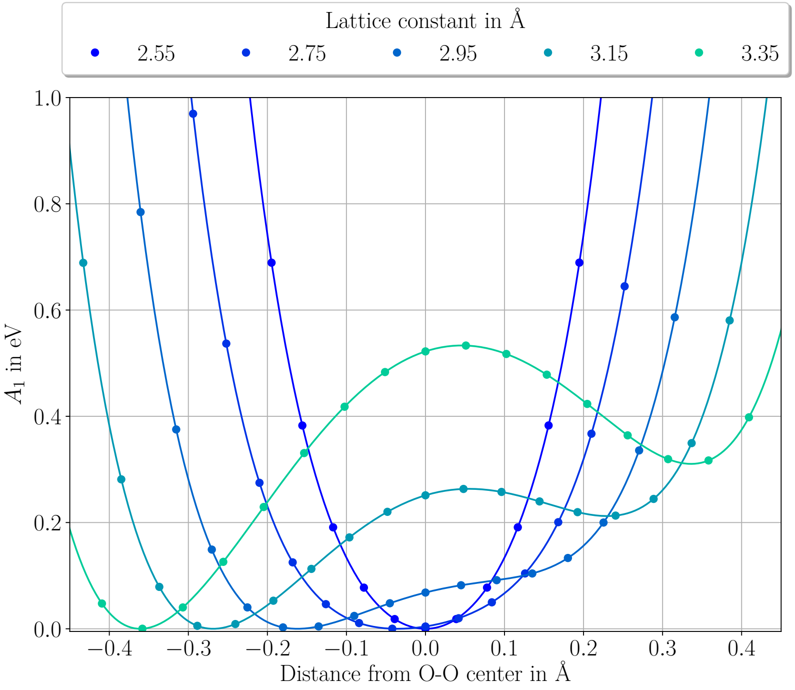


FIG. S4. Potential of proton positions along dOOd, when the ice rules are violated with (**top**) cis-$H_3O^+$ and (**bottom**) trans-$H_3O^+$ configurations (charge defects conjugated). The potentials show a significantly lower barrier than the collectively all or hexagonal configurations, and loose the double-well character at $l \lesssim 2.85$ Å. The trans-$H_3O^+$ configuration shows a more asymmetric potential due to the position of the sampling point in the simulation cell.

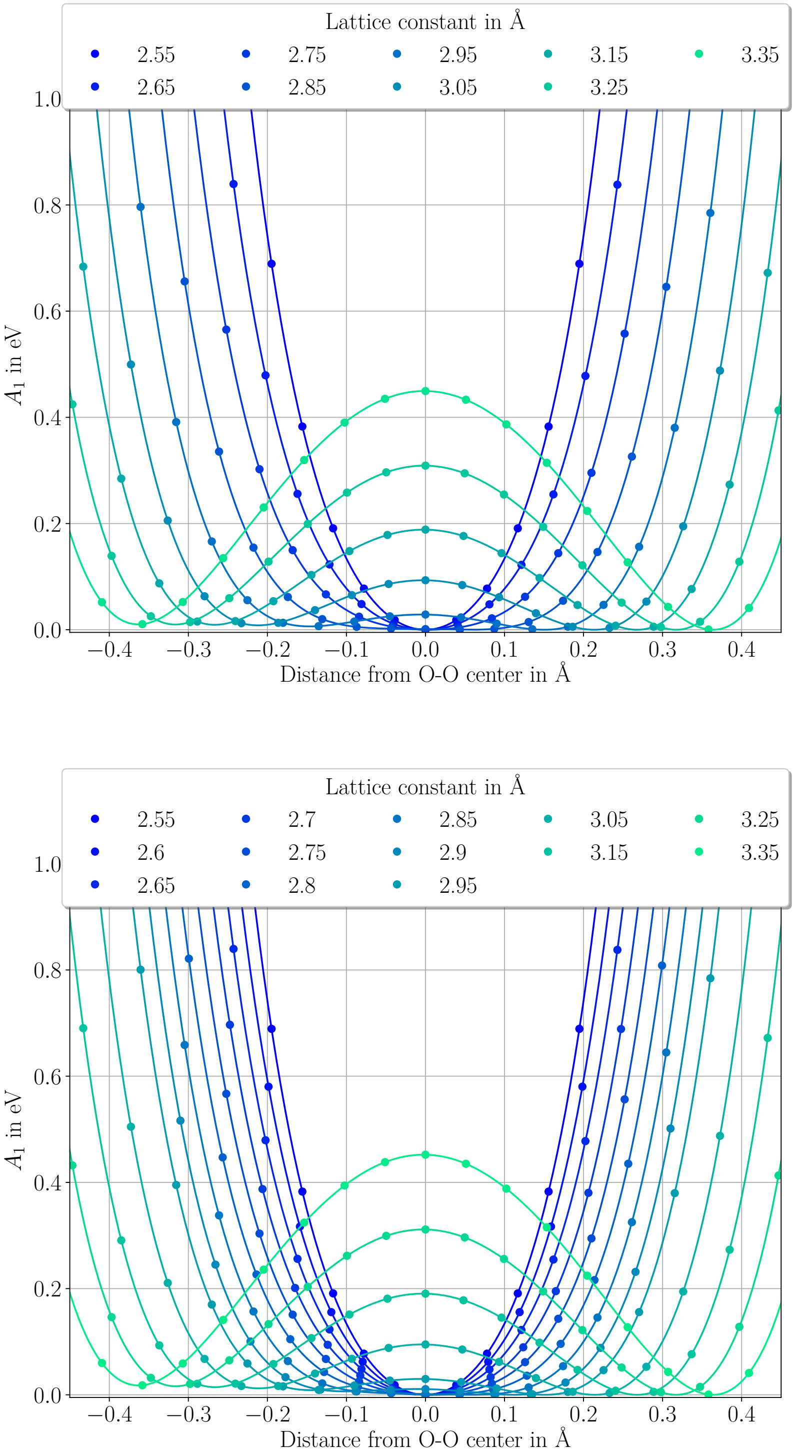


FIG. S5. Potential of proton positions along dOOd, when the ice rules are violated with (**top**) cis-$OH^-$ and (**bottom**) trans-$OH^-$ configuration (charge defects conjugated). The potentials loose the double-well character at a lattice constant of $l \lesssim 2.85$ Åin agreement with the $H_3O^+$ configurations.
